# Supplementary material for: Constraints on new vector boson mediated electron-nucleus interactions from spectroscopy of polar diatomic molecules
Source: arXiv:2503.08210 source file (2025-03-28)
Supplement: Supplementary file 1 [file suppplemental_material.pdf]

# Supplemental Material for “Constraints on new vector boson mediated electron-nucleus interactions from spectroscopy of polar diatomic molecules”

Konstantin Gaul,<sup>1,2,3,\*</sup> Lei Cong,<sup>1,2,3,†</sup> and Dmitry Budker<sup>1,2,3,4</sup>

<sup>1</sup>*Helmholtz Institut Mainz, 55099 Mainz, Germany*

<sup>2</sup>*GSI Helmholtzzentrum für Schwerionenforschung GmbH, 64291 Darmstadt, Germany*

<sup>3</sup>*Institut für Physik, Johannes Gutenberg-Universität Mainz, 55099 Mainz, Germany*

<sup>4</sup>*University of California, Berkeley, California 94720, USA*

(Dated: March 28, 2025)

## I. COMPUTATIONAL DETAILS

All calculations were performed with a modified version [1–4] of the program package [5] which is based on Turbomole [6]. Electronic densities were computed at the level of two-component zeroth order regular approximation (ZORA) within the complex generalized Kohn-Sham (cGKS) approximation. The gauge dependence of the ZORA Hamiltonian was alleviated by a model potential as suggested by van Wüllen [7] which was applied with additional damping [8]. All elements were described with the core-valence correlated basis set of quadruple zeta quality by Dyall (dyall.cv4z) [9] that was augmented for all elements with an additional set of 12 s and 6 p functions for the description of the wave function within the nucleus [dyalla.cv4z(aug)]. These additional sets of steep functions were composed as an even-tempered series starting at  $10^9 a_0^2$  and progressing by division by 1.5 for s functions and 2.5 for p functions.

Density functional theory (DFT) calculations were performed within the local density approximation (LDA) using the X $\alpha$  exchange functional [10, 11] and the VWN-5 correlation functional [12] in a hybrid LDA version with 50 % Fock exchange by Becke (BHandH) [13].

Electronic densities were optimized until the change in energy and relative spin-orbit coupling contribution was below  $10^{-10} E_h$  between two consecutive iterations.

Bond length of BaF ( $4.07 a_0$ ) and RaF ( $4.21 a_0$ ) were taken from Ref. [14]. The bond length of SiO<sup>+</sup> ( $2.84 a_0$ ) was obtained by optimization of the electronic energy up to an energy change of less than  $10^{-6} E_h$  as convergence criterion.

The nuclear magnetization and charge densities were modeled as normalized spherical Gaussian distributions  $\varrho_K(\vec{r}) = \frac{\zeta_K^{3/2}}{\pi^{3/2}} e^{-\zeta_K |\vec{r} - \vec{r}_K|^2}$  with  $\zeta_K = \frac{3}{2r_{\text{nuc},K}^2}$ . The root-mean-square radius  $r_{\text{nuc},K}$  was chosen as suggested by Visscher and Dyall employing the isotopes <sup>19</sup>F, <sup>16</sup>O, <sup>29</sup>Si, <sup>137</sup>Ba and <sup>225</sup>Ra[15]. The hyperfine coupling operator for nucleus  $K$  appears in this approximation as

$$\hat{H}_{\text{hf},K} = \frac{\mu_0}{4\pi} \sum_i^{N_{\text{elec}}} c e \vec{\alpha}_i \cdot \vec{\mathcal{A}}_K(\vec{r}_i) \quad (1)$$

where the vector potential of a spherical Gaussian nuclear magnetization distribution is

$$\vec{\mathcal{A}}_K(\vec{r}_i) = 4\sqrt{\frac{\zeta_K^3}{\pi}} \gamma_K \vec{I}_K \times (\vec{r}_i - \vec{r}_K) F_1(\zeta_K r_{iK}^2), \quad (2)$$

where  $F_n(x) = \int_0^1 dt e^{-xt^2} t^{2n}$  is the Boys function. Here and in the main text we employ standard notation for Dirac matrices, i.e.  $\vec{\alpha} = \begin{pmatrix} \mathbf{0} & \vec{\sigma} \\ \vec{\sigma} & \mathbf{0} \end{pmatrix}$  and  $\gamma^5 = \begin{pmatrix} \mathbf{0} & \mathbf{1} \\ \mathbf{1} & \mathbf{0} \end{pmatrix}$ , where  $\vec{\sigma}$  denotes the vector of Pauli spin matrices. For calculations of AV-eN magneto-gyric ratios were employed as listed in Ref. [16]:  $\gamma_{^{19}\text{F}} = 5.257736 \mu_N$ ,  $\gamma_{^{17}\text{O}} = -0.757516 \mu_N$ ,  $\gamma_{^{29}\text{Si}} = -1.11058 \mu_N$ ,  $\gamma_{^{137}\text{Ba}} = 0.624913 \mu_N$  and  $\gamma_{^{225}\text{Ra}} = -1.4676 \mu_N$ .

Standard Model PV matrix elements  $W_a$  were computed using the electroweak (ew) NSDPV operator [17]

$$\hat{H}_{\text{ew,NSDPV}} = \frac{G_F}{\sqrt{2}} \sum_i^{N_{\text{elec}}} \sum_K^{N_{\text{nuc}}} \vec{I}_K \cdot \vec{\alpha}_i \rho_K(\vec{r}_i), \quad (3)$$

---

\* konstantin.gaul@uni-mainz.de

† conglei1@uni-mainz.de

which differs only by a constant factor from  $\lim_{M \rightarrow \infty} \hat{H}_{\text{AV-Ne}}$ . Here  $G_F \approx 2.22249 E_h a_0^3$  is Fermi's weak coupling constant. For the ZORA form of this operator see Ref. [18–20]. In the present work all molecular properties were computed with the toolbox approach presented in Ref. [1]. In this approach the transformation from the four-component picture to the 2c-ZORA picture is automatic.

To compute spin-polarized off-diagonal  $\Omega$  matrix elements, we optimized the electronic density with the electronic total angular momentum being orthogonal to the molecular axis as done previously in the computation of g-tensors [21] and hyperfine coupling constants [19, 20, 22] with similar methods :

$$\langle \Omega | \hat{H}_{\text{NSDPV}} | -\Omega \rangle / \Omega = \langle \Psi_{\vec{J}_e \perp \vec{\lambda}} | \hat{H}_{\text{NSDPV}, \parallel \vec{J}_e \times \vec{\lambda}} | \Psi_{\vec{J}_e \perp \vec{\lambda}} \rangle / \Omega \quad (4)$$

where  $\parallel \vec{J}_e \times \vec{\lambda}$  denotes that the component of  $\hat{H}_{\text{NSDPV}}$ , which is orthogonal to  $\vec{J}_e$  and  $\vec{\lambda}$ . In our calculation we took  $\vec{\lambda}$  to be aligned along the  $z$ -axis and  $\vec{J}_e$  to be aligned along the  $x$ -axis. Thus, in our calculations only the  $y$ -component of  $\hat{H}_{\text{NSDPV}}$  is non-zero. In this approach no rescaling of  $W_a$  with hyperfine-coupling spin polarization as suggested in Ref. [19] is required.

In case of AV-eN interactions the second order expression appears within HF theory and DFT as linear response function for the  $|\Psi_{\vec{J}_e \perp \vec{\lambda}}\rangle$  wave function as

$$W_{\text{AV-eN}} = \left\langle \left\langle \hat{H}_{\text{AV-eN}}; \hat{H}_{\text{hf}, \parallel \vec{J}_e \times \vec{\lambda}} \right\rangle \right\rangle_{\vec{J}_e \perp \vec{\lambda}} / \Omega, \quad (5)$$

where  $\langle \langle \hat{A}; \hat{B} \rangle \rangle$  denotes the linear response function of operator  $\hat{A}$  under perturbation of operator  $\hat{B}$ . The ZORA form of the effective electroweak  $\hat{H}_{\text{AV-eN}}$ -type operator was derived in Ref. [23]. All resulting coupled perturbed (CP) Kohn-Sham (CPKS) equations were solved in a conjugate gradients algorithm as described in Refs. [2, 4]. We provide for comparison also values for the uncoupled (UC) Kohn-Sham results, which correspond to a simple sum-over-states expression involving only unperturbed KS orbitals. Within ZORA the second-order property  $W_{\text{AV-eN}}$  has a diamagnetic-like contribution (dia), because of the transformation from the four-component to the two-component picture (see Ref. [20] for the diamagnetic-like ZORA operator of the electroweak interaction), which is computed as an expectation value of an operator that is bilinear in the nuclear spin and electron spin:

$$H_{\text{hf,AV-eN,dia}}^{\text{ZORA}} = \frac{\hbar c \mu_0}{4\pi^2} \sum_i^{N_{\text{elec}}} \sum_K^{N_{\text{nuc}}} A_K \vec{\sigma} \cdot \vec{\mathcal{A}}_K(\vec{r}_i) \omega(\vec{r}_i) V_{Y,K}(\vec{r}_i), \quad (6)$$

where  $\omega(\vec{r}_i) = \frac{1}{2m_e c^2 - \tilde{V}(\vec{r}_i)}$  is the ZORA factor with van Wüllen's model potential being  $\tilde{V}$ .

In the current implementation [1] the Yukawa potential is only available for a point-like nucleus. However, the contact-like interaction for masses  $M \rightarrow \infty$  as well as for  $M \rightarrow 0$  can be evaluated for different nuclear models. We studied the effect of a finite nuclear size by computing the limits  $M \rightarrow 0$  and  $M \rightarrow \infty$  for a point-like nucleus and a finite, spherical Gaussian nuclear density distribution. For the former model the Yukawa-like operator reduces to  $\lim_{M \rightarrow \infty} V_{Y,K} = \hbar^2 4\pi \delta^3(r_{iK}) / (Mc)^2$  and  $\lim_{M \rightarrow 0} V_{Y,K} = \frac{1}{r_{iK}}$  and for the latter it reduces to

$\lim_{M \rightarrow 0} V_{Y,K} = \hbar^2 4\pi \rho_K(r_{iK}) / (Mc)^2$  and  $\lim_{M \rightarrow \infty} V_{Y,K} = \frac{\text{erf}(\sqrt{\zeta_K} r_{iK})}{r_{iK}}$ , respectively. The results for the limits  $M \rightarrow 0$  and  $M \rightarrow \infty$  are compared in the Sec. II.

Results for electroweak PV matrix elements  $W_a$  as well as for matrix elements of AV-Ne interactions in the limit  $M \rightarrow \infty$ , which were used for calculations of interactions of electrons with nuclear anapole moments due to a new boson, are presented in the main text for the finite nuclear model.

## II. NUMERICAL RESULTS, INFLUENCE OF FINITE NUCLEAR SIZE EFFECTS, COMPUTATIONAL ACCURACY

Results of PV matrix elements that mix  $\Omega$  states are shown for  $\text{Ba}^{19}\text{F}$  in Table I,  $^{137}\text{BaF}$  in Table II,  $\text{Ra}^{19}\text{F}$  in Table III,  $^{225}\text{RaF}$  in Table IV,  $\text{Si}^{17}\text{O}^+$  in Table V and  $^{29}\text{SiO}^+$  in Table VI.

In the limit  $M \rightarrow 0$  the results of calculations with finite nucleus (GN) and a point-like nucleus (PN) are essentially identical. Therefore, we consider the error of Yukawa-like interactions computed for boson masses  $M < 10 \text{ keV}/c^2$  to be negligible. The error is much more pronounced in the limit  $M \rightarrow \infty$ , where it reaches for  $^{225}\text{RaF}$  up to 20 % for AV-Ne and 40 % for AV-eN interactions. For example, the sensitivity to AV-eN for boson mass  $5.11 \times 10^9$  changes

Table I. Parity-violating matrix elements that mix  $|\Omega\rangle$  and  $|- \Omega\rangle$  states in  $\text{Ba}^{19}\text{F}$  from electron- $^{19}\text{F}$  interactions for different boson masses  $M$  at the level of 2c-ZORA-BHandH/dyall.cv4z(aug). In the limits  $M \rightarrow 0$  and  $M \rightarrow \infty$ , results are shown for a Gaussian (GN) and point-like (PN) nuclear charge density distribution. For AV-eN interactions diamagnetic-like expectation value contributions  $W_{\text{AV-eN,dia}}$ , uncoupled  $W_{\text{AV-eN,UC}}$  and coupled-perturbed results  $W_{\text{AV-eN,CP}}$  are shown (see text in Sec.II) for details). Standard Model electroweak contributions to the parity-violating matrix elements  $W_a$  can be obtained from results for  $W_{\text{AV-Ne}}$  (GN) in the limit  $M \rightarrow \infty$  by multiplication with  $\frac{G_F}{\sqrt{2}h^3c^3}$ . For AV-eN interaction matrix elements we used  $\gamma_{^{19}\text{F}} = 5.257736 \mu_N$ .

| $Mc^2/\text{eV}$      | $W_{\text{AV-Ne}}/(h \text{ Hz})$                     | $W_{\text{AV-eN,dia}}/(h \text{ Hz})$                     | $W_{\text{AV-eN,UC}}/(h \text{ Hz})$                     | $W_{\text{AV-eN,CP}}/(h \text{ Hz})$                     |
|-----------------------|-------------------------------------------------------|-----------------------------------------------------------|----------------------------------------------------------|----------------------------------------------------------|
| 0 (GN)                | $-9.56 \times 10^{12}$                                | $2.01 \times 10^6$                                        | $1.65 \times 10^8$                                       | $6.64 \times 10^8$                                       |
| 0 (PN)                | $-9.56 \times 10^{12}$                                | $2.01 \times 10^6$                                        | $1.65 \times 10^8$                                       | $6.65 \times 10^8$                                       |
| $5.11 \times 10^{-5}$ | $-9.56 \times 10^{12}$                                | $2.01 \times 10^6$                                        | $1.65 \times 10^8$                                       | $6.64 \times 10^8$                                       |
| $5.11 \times 10^{-3}$ | $-9.56 \times 10^{12}$                                | $2.01 \times 10^6$                                        | $1.65 \times 10^8$                                       | $6.64 \times 10^8$                                       |
| $5.11 \times 10^{-1}$ | $-9.56 \times 10^{12}$                                | $2.01 \times 10^6$                                        | $1.65 \times 10^8$                                       | $6.64 \times 10^8$                                       |
| $5.11 \times 10^1$    | $-9.52 \times 10^{12}$                                | $2.38 \times 10^6$                                        | $1.57 \times 10^8$                                       | $6.30 \times 10^8$                                       |
| $2.55 \times 10^2$    | $-8.90 \times 10^{12}$                                | $3.60 \times 10^6$                                        | $1.28 \times 10^8$                                       | $5.16 \times 10^8$                                       |
| $5.11 \times 10^2$    | $-7.60 \times 10^{12}$                                | $4.67 \times 10^6$                                        | $1.02 \times 10^8$                                       | $4.09 \times 10^8$                                       |
| $2.55 \times 10^3$    | $-1.25 \times 10^{12}$                                | $7.10 \times 10^6$                                        | $3.71 \times 10^7$                                       | $1.29 \times 10^8$                                       |
| $5.11 \times 10^3$    | $-1.67 \times 10^{11}$                                | $7.40 \times 10^6$                                        | $2.68 \times 10^7$                                       | $7.97 \times 10^7$                                       |
| $2.55 \times 10^4$    | $1.73 \times 10^{11}$                                 | $6.31 \times 10^6$                                        | $7.11 \times 10^2$                                       | $1.53 \times 10^7$                                       |
| $5.11 \times 10^4$    | $1.46 \times 10^{11}$                                 | $4.88 \times 10^6$                                        | $-8.32 \times 10^6$                                      | $-1.04 \times 10^6$                                      |
| $2.55 \times 10^5$    | $2.28 \times 10^{10}$                                 | $1.60 \times 10^6$                                        | $-5.91 \times 10^6$                                      | $-5.27 \times 10^6$                                      |
| $5.11 \times 10^5$    | $7.00 \times 10^9$                                    | $8.40 \times 10^5$                                        | $-3.59 \times 10^6$                                      | $-3.41 \times 10^6$                                      |
| $5.11 \times 10^6$    | $7.07 \times 10^7$                                    | $7.27 \times 10^4$                                        | $-1.06 \times 10^6$                                      | $-1.06 \times 10^6$                                      |
| $5.11 \times 10^7$    | $6.21 \times 10^5$                                    | $4.00 \times 10^3$                                        | $-2.59 \times 10^5$                                      | $-2.59 \times 10^5$                                      |
| $5.11 \times 10^9$    | $6.17 \times 10^1$                                    | $1.32 \times 10^{-3}$                                     | $-6.65 \times 10^1$                                      | $-6.65 \times 10^1$                                      |
| $5.11 \times 10^{11}$ | $6.16 \times 10^{-3}$                                 | $1.32 \times 10^{-11}$                                    | $-6.65 \times 10^{-3}$                                   | $-6.65 \times 10^{-3}$                                   |
| $5.11 \times 10^{13}$ | $6.16 \times 10^{-7}$                                 | $1.32 \times 10^{-19}$                                    | $-6.65 \times 10^{-7}$                                   | $-6.65 \times 10^{-7}$                                   |
| <hr/>                 |                                                       |                                                           |                                                          |                                                          |
|                       | $W_{\text{AV-Ne}} M^2 c^4/(\text{eV}^2 h \text{ Hz})$ | $W_{\text{AV-eN,dia}} M^2 c^4/(\text{eV}^2 h \text{ Hz})$ | $W_{\text{AV-eN,UC}} M^2 c^4/(\text{eV}^2 h \text{ Hz})$ | $W_{\text{AV-eN,CP}} M^2 c^4/(\text{eV}^2 h \text{ Hz})$ |
| $\infty$ (PN)         | $1.61 \times 10^{21}$                                 | 0                                                         | $-1.74 \times 10^{21}$                                   | $-1.74 \times 10^{21}$                                   |
| $\infty$ (GN)         | $1.74 \times 10^{21}$                                 | $1.30 \times 10^{19}$                                     | $-1.51 \times 10^{21}$                                   | $-1.51 \times 10^{21}$                                   |

from  $-1.8 \times 10^{-7} h \text{ Hz}$  to  $-2.5 \times 10^{-7} h \text{ Hz}$  considering the finite size of the nucleus. This error will, thus, not affect the order of magnitude of bounds discussed in the main text and will be hardly visible in Fig. 2 of the main text.

Moreover, we note by comparison of CP and UC results that response effects from the CPKS equation are negligible for boson masses  $M > \text{MeV}/c^2$ , whereas they are very important for smaller boson masses. Moreover, we note that in case of BaF CPKS equations converged only very slowly, indicating strong correlation effects. Therefore, we consider the reported values for AV-eN interactions for boson masses  $M < \text{MeV}/c^2$  less accurate than those for larger boson masses.

In case of AV-Ne interactions an excellent agreement of electroweak PV matrix elements with sophisticated four-component relativistic coupled cluster calculations is found (see main text). This suggests that the accuracy of our calculations of AV-Ne calculations for masses  $M < 10 \text{ keV}$  is better than 10 % for heavy nucleus PV as in  $^{137}\text{BaF}$  and  $^{225}\text{RaF}$  and better than 20 % for lighter nuclei.

- 
- [1] K. Gaul and R. Berger, Toolbox approach for quasi-relativistic calculation of molecular properties for precision tests of fundamental physics, J. Chem. Phys. **152**, 044101 (2020).
  - [2] M. T. Colombo Jofré, K. Koziół, I. A. Aucar, K. Gaul, R. Berger, and G. A. Aucar, Relativistic and QED corrections to one-bond indirect nuclear spin-spin couplings in  $\text{X}_2^{2+}$  and  $\text{X}_3^{2+}$  ions ( $\text{X} = \text{Zn}, \text{Cd}, \text{Hg}$ ), J. Chem. Phys. **157**, 064103 (2022).
  - [3] C. Zülch, K. Gaul, S. M. Giesen, R. F. G. Ruiz, and R. Berger, Cool molecular highly charged ions for precision tests of fundamental physics, arXiv **physics.chem-ph**, 2203.10333 (2022).
  - [4] S. A. Brück, N. Sahu, K. Gaul, and R. Berger, Quasi-relativistic approach to analytical gradients of parity violating potentials, J. Chem. Phys. **158**, 194109 (2023).
  - [5] C. van Wüllen, A Quasirelativistic Two-component Density Functional and Hartree-Fock Program, Z. Phys. Chem **224**, 413 (2010).
  - [6] R. Ahlrichs, M. Bär, M. Häser, H. Horn, and C. Kölmel, Electronic structure calculations on workstation computers: The

Table II. Parity-violating matrix elements that mix  $|\Omega\rangle$  and  $|\Omega\rangle$  states in  $^{137}\text{BaF}$  from electron- $^{137}\text{Ba}$  interactions for different boson masses  $M$  at the level of 2c-ZORA-BHandH/dyall.cv4z(aug). In the limits  $M \rightarrow 0$  and  $M \rightarrow \infty$ , results are shown for a Gaussian (GN) and point-like (PN) nuclear charge density distribution. For AV-eN interactions diamagnetic-like expectation value contributions  $W_{\text{AV-eN,dia}}$ , uncoupled  $W_{\text{AV-eN,UC}}$  and coupled-perturbed results  $W_{\text{AV-eN,CP}}$  are shown (see text in Sec.II) for details). Standard Model electroweak contributions to the parity-violating matrix elements  $W_a$  can be obtained from results for  $W_{\text{AV-Ne}}$  (GN) in the limit  $M \rightarrow \infty$  by multiplication with  $\frac{G_F}{\sqrt{2}h^3c^3}$ . For AV-eN interaction matrix elements we used  $\gamma_{^{137}\text{Ba}} = 0.624913 \mu\text{N}$ .

| $Mc^2/\text{eV}$      | $W_{\text{AV-Ne}}/(h \text{ Hz})$                     | $W_{\text{AV-eN,dia}}/(h \text{ Hz})$                     | $W_{\text{AV-eN,UC}}/(h \text{ Hz})$                     | $W_{\text{AV-eN,CP}}/(h \text{ Hz})$                     |
|-----------------------|-------------------------------------------------------|-----------------------------------------------------------|----------------------------------------------------------|----------------------------------------------------------|
| 0 (GN)                | $-7.87 \times 10^{12}$                                | $4.92 \times 10^9$                                        | $5.73 \times 10^9$                                       | $-2.62 \times 10^9$                                      |
| 0 (PN)                | $-7.87 \times 10^{12}$                                | $4.92 \times 10^9$                                        | $5.47 \times 10^9$                                       | $-2.88 \times 10^9$                                      |
| $5.11 \times 10^{-5}$ | $-7.87 \times 10^{12}$                                | $4.92 \times 10^9$                                        | $5.47 \times 10^9$                                       | $-2.93 \times 10^9$                                      |
| $5.11 \times 10^{-3}$ | $-7.87 \times 10^{12}$                                | $4.92 \times 10^9$                                        | $5.47 \times 10^9$                                       | $-2.93 \times 10^9$                                      |
| $5.11 \times 10^{-1}$ | $-7.87 \times 10^{12}$                                | $4.92 \times 10^9$                                        | $5.47 \times 10^9$                                       | $-2.94 \times 10^9$                                      |
| $5.11 \times 10^1$    | $-7.85 \times 10^{12}$                                | $4.93 \times 10^9$                                        | $4.95 \times 10^9$                                       | $-3.16 \times 10^9$                                      |
| $2.55 \times 10^2$    | $-7.60 \times 10^{12}$                                | $4.93 \times 10^9$                                        | $3.07 \times 10^9$                                       | $-3.81 \times 10^9$                                      |
| $5.11 \times 10^2$    | $-7.00 \times 10^{12}$                                | $4.93 \times 10^9$                                        | $1.12 \times 10^9$                                       | $-4.19 \times 10^9$                                      |
| $2.55 \times 10^3$    | $-2.07 \times 10^{12}$                                | $4.94 \times 10^9$                                        | $-6.79 \times 10^9$                                      | $-2.35 \times 10^9$                                      |
| $5.11 \times 10^3$    | $8.65 \times 10^{11}$                                 | $4.94 \times 10^9$                                        | $-1.08 \times 10^{10}$                                   | $-6.69 \times 10^8$                                      |
| $2.55 \times 10^4$    | $7.71 \times 10^{12}$                                 | $4.87 \times 10^9$                                        | $-2.04 \times 10^{10}$                                   | $-9.67 \times 10^9$                                      |
| $5.11 \times 10^4$    | $1.03 \times 10^{13}$                                 | $4.73 \times 10^9$                                        | $-2.40 \times 10^{10}$                                   | $-1.87 \times 10^{10}$                                   |
| $2.55 \times 10^5$    | $1.19 \times 10^{13}$                                 | $3.59 \times 10^9$                                        | $-2.54 \times 10^{10}$                                   | $-2.77 \times 10^{10}$                                   |
| $5.11 \times 10^5$    | $8.48 \times 10^{12}$                                 | $2.70 \times 10^9$                                        | $-2.12 \times 10^{10}$                                   | $-2.28 \times 10^{10}$                                   |
| $5.11 \times 10^6$    | $3.99 \times 10^{11}$                                 | $4.93 \times 10^8$                                        | $-5.98 \times 10^9$                                      | $-6.03 \times 10^9$                                      |
| $5.11 \times 10^7$    | $6.53 \times 10^9$                                    | $2.22 \times 10^7$                                        | $-6.49 \times 10^8$                                      | $-6.50 \times 10^8$                                      |
| $5.11 \times 10^9$    | $7.41 \times 10^5$                                    | $2.32$                                                    | $-1.09 \times 10^5$                                      | $-1.09 \times 10^5$                                      |
| $5.11 \times 10^{11}$ | $7.41 \times 10^1$                                    | $2.32 \times 10^{-8}$                                     | $-1.09 \times 10^1$                                      | $-1.09 \times 10^1$                                      |
| $5.11 \times 10^{13}$ | $7.41 \times 10^{-3}$                                 | $2.32 \times 10^{-16}$                                    | $-1.09 \times 10^{-3}$                                   | $-1.09 \times 10^{-3}$                                   |
| <hr/>                 |                                                       |                                                           |                                                          |                                                          |
|                       | $W_{\text{AV-Ne}} M^2 c^4/(\text{eV}^2 h \text{ Hz})$ | $W_{\text{AV-eN,dia}} M^2 c^4/(\text{eV}^2 h \text{ Hz})$ | $W_{\text{AV-eN,UC}} M^2 c^4/(\text{eV}^2 h \text{ Hz})$ | $W_{\text{AV-eN,CP}} M^2 c^4/(\text{eV}^2 h \text{ Hz})$ |
| $\infty$ (PN)         | $1.94 \times 10^{25}$                                 | 0                                                         | $-2.85 \times 10^{24}$                                   | $-2.85 \times 10^{24}$                                   |
| $\infty$ (GN)         | $1.81 \times 10^{25}$                                 | $6.31 \times 10^{22}$                                     | $-2.25 \times 10^{24}$                                   | $-2.25 \times 10^{24}$                                   |

program system turbomole, Chem. Phys. Lett. **162**, 165 (1989).

- [7] C. van Wüllen, Molecular density functional calculations in the regular relativistic approximation: Method, application to coinage metal diatomics, hydrides, fluorides and chlorides, and comparison with first-order relativistic calculations, J. Chem. Phys. **109**, 392 (1998).
- [8] W. Liu, C. van Wüllen, F. Wang, and L. Li, Spectroscopic constants of MH and M<sub>2</sub> (M = Tl, E113, Bi, E115): direct comparisons of four- and two-component approaches in the framework of relativistic density functional theory, J. Chem. Phys. **116**, 3626 (2002).
- [9] K. G. Dyall, Relativistic quadruple-zeta and revised triple-zeta and double-zeta basis sets for the 4p, 5p, and 6p elements, Theor. Chem. Acc. **115**, 441 (2006).
- [10] P. A. M. Dirac, Note on exchange phenomena in the Thomas atom, Proc. Cambridge Phil. Soc. **26**, 376 (1930).
- [11] J. C. Slater, A simplification of the Hartree-Fock method, Phys. Rev. **81**, 385 (1951).
- [12] S. H. Vosko, L. Wilk, and M. Nuisar, Accurate spin-dependent electron liquid correlation energies for local spin density calculations: A critical analysis, Can. J. Phys. **58**, 1200 (1980).
- [13] A. D. Becke, A new mixing of Hartree-Fock and local density-functional theories, J. Chem. Phys. **98**, 1372 (1993).
- [14] K. Gaul and R. Berger, Global analysis of  $\mathcal{CP}$ -violation in atoms, molecules and role of medium-heavy systems, J. High Energ. Phys. **2024** (8), 100.
- [15] L. Visscher and K. G. Dyall, Dirac-fock atomic electronic structure calculations using different nuclear charge distributions, At. Data Nucl. Data Tables **67**, 207 (1997).
- [16] N. Stone, Table of nuclear magnetic dipole and electric quadrupole moments, At. Data Nucl. Data Tables **90**, 75 (2005).
- [17] A. Moskalev, R. Ryndin, and I. Khriplovich, On the possibility of weak interaction investigation in atomic physics, Uspekhi. Phys. **118**, 409 (1976).
- [18] S. Nahrwold and R. Berger, Zeroth order regular approximation approach to parity violating nuclear magnetic resonance shielding tensors, J. Chem. Phys. **130**, 214101 (2009).
- [19] T. A. Isaev, S. Hoekstra, and R. Berger, Laser-cooled RaF as a promising candidate to measure molecular parity violation, Phys. Rev. A **82**, 052521 (2010).
- [20] T. A. Isaev and R. Berger, Electron correlation and nuclear charge dependence of parity-violating properties in open-shell diatomic molecules, Phys. Rev. A **86**, 062515 (2012).
- [21] I. Malkin, O. L. Malkina, V. G. Malkin, and M. Kaupp, Relativistic two-component calculations of electronic

Table III. Parity-violating matrix elements that mix  $|\Omega\rangle$  and  $|- \Omega\rangle$  states in  $\text{Ra}^{19}\text{F}$  from electron- $^{19}\text{F}$  interactions for different boson masses  $M$  at the level of 2c-ZORA-BHandH/dyall.cv4z(aug). In the limits  $M \rightarrow 0$  and  $M \rightarrow \infty$ , results are shown for a Gaussian (GN) and point-like (PN) nuclear charge density distribution. For AV-eN interactions diamagnetic-like expectation value contributions  $W_{\text{AV-eN,dia}}$ , uncoupled  $W_{\text{AV-eN,UC}}$  and coupled-perturbed results  $W_{\text{AV-eN,CP}}$  are shown (see text in Sec.II) for details). Standard Model electroweak contributions to the parity-violating matrix elements  $W_a$  can be obtained from results for  $W_{\text{AV-Ne}}$  (GN) in the limit  $M \rightarrow \infty$  by multiplication with  $\frac{G_F}{\sqrt{2}h^3c^3}$ . For AV-eN interaction matrix elements we used  $\gamma_{^{19}\text{F}} = 5.257736 \mu_N$ .

| $Mc^2/\text{eV}$      | $W_{\text{AV-Ne}}/(h \text{ Hz})$                     | $W_{\text{AV-eN,dia}}/(h \text{ Hz})$                     | $W_{\text{AV-eN,UC}}/(h \text{ Hz})$                     | $W_{\text{AV-eN,CP}}/(h \text{ Hz})$                     |
|-----------------------|-------------------------------------------------------|-----------------------------------------------------------|----------------------------------------------------------|----------------------------------------------------------|
| 0 (GN)                | $-1.01 \times 10^{13}$                                | $4.55 \times 10^7$                                        | $2.82 \times 10^8$                                       | $5.13 \times 10^8$                                       |
| 0 (PN)                | $-1.01 \times 10^{13}$                                | $4.55 \times 10^7$                                        | $2.82 \times 10^8$                                       | $5.13 \times 10^8$                                       |
| $5.11 \times 10^{-5}$ | $-1.01 \times 10^{13}$                                | $4.55 \times 10^7$                                        | $2.82 \times 10^8$                                       | $5.13 \times 10^8$                                       |
| $5.11 \times 10^{-3}$ | $-1.01 \times 10^{13}$                                | $4.55 \times 10^7$                                        | $2.82 \times 10^8$                                       | $5.13 \times 10^8$                                       |
| $5.11 \times 10^{-1}$ | $-1.01 \times 10^{13}$                                | $4.55 \times 10^7$                                        | $2.81 \times 10^8$                                       | $5.13 \times 10^8$                                       |
| $5.11 \times 10^1$    | $-1.00 \times 10^{13}$                                | $4.59 \times 10^7$                                        | $2.70 \times 10^8$                                       | $4.92 \times 10^8$                                       |
| $2.55 \times 10^2$    | $-9.39 \times 10^{12}$                                | $4.73 \times 10^7$                                        | $2.30 \times 10^8$                                       | $4.24 \times 10^8$                                       |
| $5.11 \times 10^2$    | $-8.07 \times 10^{12}$                                | $4.85 \times 10^7$                                        | $1.94 \times 10^8$                                       | $3.62 \times 10^8$                                       |
| $2.55 \times 10^3$    | $-1.47 \times 10^{12}$                                | $5.13 \times 10^7$                                        | $9.27 \times 10^7$                                       | $2.20 \times 10^8$                                       |
| $5.11 \times 10^3$    | $-1.52 \times 10^{11}$                                | $5.15 \times 10^7$                                        | $5.85 \times 10^7$                                       | $1.92 \times 10^8$                                       |
| $2.55 \times 10^4$    | $9.92 \times 10^{11}$                                 | $4.29 \times 10^7$                                        | $-6.66 \times 10^7$                                      | $2.01 \times 10^7$                                       |
| $5.11 \times 10^4$    | $8.66 \times 10^{11}$                                 | $3.31 \times 10^7$                                        | $-8.92 \times 10^7$                                      | $-4.16 \times 10^7$                                      |
| $2.55 \times 10^5$    | $1.41 \times 10^{11}$                                 | $1.08 \times 10^7$                                        | $-4.06 \times 10^7$                                      | $-3.59 \times 10^7$                                      |
| $5.11 \times 10^5$    | $4.34 \times 10^{10}$                                 | $5.66 \times 10^6$                                        | $-2.33 \times 10^7$                                      | $-2.20 \times 10^7$                                      |
| $5.11 \times 10^6$    | $4.40 \times 10^8$                                    | $4.80 \times 10^5$                                        | $-6.45 \times 10^6$                                      | $-6.44 \times 10^6$                                      |
| $5.11 \times 10^7$    | $3.72 \times 10^6$                                    | $2.42 \times 10^4$                                        | $-1.49 \times 10^6$                                      | $-1.49 \times 10^6$                                      |
| $5.11 \times 10^9$    | $3.06 \times 10^2$                                    | $6.42 \times 10^{-3}$                                     | $-3.46 \times 10^2$                                      | $-3.46 \times 10^2$                                      |
| $5.11 \times 10^{11}$ | $3.06 \times 10^{-2}$                                 | $6.41 \times 10^{-11}$                                    | $-3.46 \times 10^{-2}$                                   | $-3.46 \times 10^{-2}$                                   |
| $5.11 \times 10^{13}$ | $3.06 \times 10^{-6}$                                 | $6.41 \times 10^{-19}$                                    | $-3.46 \times 10^{-6}$                                   | $-3.46 \times 10^{-6}$                                   |
| <hr/>                 |                                                       |                                                           |                                                          |                                                          |
|                       | $W_{\text{AV-Ne}} M^2 c^4/(\text{eV}^2 h \text{ Hz})$ | $W_{\text{AV-eN,dia}} M^2 c^4/(\text{eV}^2 h \text{ Hz})$ | $W_{\text{AV-eN,UC}} M^2 c^4/(\text{eV}^2 h \text{ Hz})$ | $W_{\text{AV-eN,CP}} M^2 c^4/(\text{eV}^2 h \text{ Hz})$ |
| $\infty$ (PN)         | $7.98 \times 10^{21}$                                 | 0                                                         | $-9.03 \times 10^{21}$                                   | $-9.03 \times 10^{21}$                                   |
| $\infty$ (GN)         | $9.75 \times 10^{21}$                                 | $7.26 \times 10^{19}$                                     | $-8.48 \times 10^{21}$                                   | $-8.48 \times 10^{21}$                                   |

g-tensors that include spin polarization, J. Chem. Phys. **123**, 244103 (2005), [https://pubs.aip.org/aip/jcp/article-pdf/doi/10.1063/1.2135290/13513718/244103\\_1.online.pdf](https://pubs.aip.org/aip/jcp/article-pdf/doi/10.1063/1.2135290/13513718/244103_1.online.pdf).

- [22] K. Gaul and R. Berger, Ab initio study of parity and time-reversal violation in laser-coolable triatomic molecules, Phys. Rev. A **101**, 012508 (2020).
- [23] R. Berger, N. Langermann, and C. van Wüllen, Zeroth order regular approximation approach to molecular parity violation, Phys. Rev. A **71**, 042105 (2005).

Table IV. Parity-violating matrix elements that mix  $|\Omega\rangle$  and  $|- \Omega\rangle$  states in  $^{225}\text{RaF}$  from electron- $^{225}\text{Ra}$  interactions for different boson masses  $M$  at the level of 2c-ZORA-BHandH/dyall.cv4z(aug). In the limits  $M \rightarrow 0$  and  $M \rightarrow \infty$ , results are shown for a Gaussian (GN) and point-like (PN) nuclear charge density distribution. For AV-eN interactions diamagnetic-like expectation value contributions  $W_{\text{AV-eN,dia}}$ , uncoupled  $W_{\text{AV-eN,UC}}$  and coupled-perturbed results  $W_{\text{AV-eN,CP}}$  are shown (see text in Sec.II) for details). Standard Model electroweak contributions to the parity-violating matrix elements  $W_a$  can be obtained from results for  $W_{\text{AV-Ne}}$  (GN) in the limit  $M \rightarrow \infty$  by multiplication with  $\frac{G_F}{\sqrt{2}h^3c^3}$ . For AV-eN interaction matrix elements we used  $\gamma_{^{225}\text{Ra}} = -1.4676 \mu_N$ .

| $Mc^2/\text{eV}$      | $W_{\text{AV-Ne}}/(h \text{ Hz})$                     | $W_{\text{AV-eN,dia}}/(h \text{ Hz})$                     | $W_{\text{AV-eN,UC}}/(h \text{ Hz})$                     | $W_{\text{AV-eN,CP}}/(h \text{ Hz})$                     |
|-----------------------|-------------------------------------------------------|-----------------------------------------------------------|----------------------------------------------------------|----------------------------------------------------------|
| 0 (GN)                | $9.75 \times 10^{12}$                                 | $-6.81 \times 10^{10}$                                    | $1.71 \times 10^{11}$                                    | $1.16 \times 10^{11}$                                    |
| 0 (PN)                | $9.78 \times 10^{12}$                                 | $-6.83 \times 10^{10}$                                    | $1.83 \times 10^{11}$                                    | $1.28 \times 10^{11}$                                    |
| $5.11 \times 10^{-5}$ | $9.78 \times 10^{12}$                                 | $-6.83 \times 10^{10}$                                    | $1.83 \times 10^{11}$                                    | $1.28 \times 10^{11}$                                    |
| $5.11 \times 10^{-3}$ | $9.78 \times 10^{12}$                                 | $-6.83 \times 10^{10}$                                    | $1.83 \times 10^{11}$                                    | $1.28 \times 10^{11}$                                    |
| $5.11 \times 10^{-1}$ | $9.78 \times 10^{12}$                                 | $-6.83 \times 10^{10}$                                    | $1.83 \times 10^{11}$                                    | $1.28 \times 10^{11}$                                    |
| $5.11 \times 10^1$    | $9.79 \times 10^{12}$                                 | $-6.83 \times 10^{10}$                                    | $1.89 \times 10^{11}$                                    | $1.40 \times 10^{11}$                                    |
| $2.55 \times 10^2$    | $1.00 \times 10^{13}$                                 | $-6.83 \times 10^{10}$                                    | $2.12 \times 10^{11}$                                    | $1.83 \times 10^{11}$                                    |
| $5.11 \times 10^2$    | $1.05 \times 10^{13}$                                 | $-6.83 \times 10^{10}$                                    | $2.35 \times 10^{11}$                                    | $2.26 \times 10^{11}$                                    |
| $2.55 \times 10^3$    | $1.45 \times 10^{13}$                                 | $-6.83 \times 10^{10}$                                    | $3.33 \times 10^{11}$                                    | $3.83 \times 10^{11}$                                    |
| $5.11 \times 10^3$    | $1.65 \times 10^{13}$                                 | $-6.83 \times 10^{10}$                                    | $3.83 \times 10^{11}$                                    | $4.49 \times 10^{11}$                                    |
| $2.55 \times 10^4$    | $2.00 \times 10^{13}$                                 | $-6.79 \times 10^{10}$                                    | $5.06 \times 10^{11}$                                    | $5.85 \times 10^{11}$                                    |
| $5.11 \times 10^4$    | $2.12 \times 10^{13}$                                 | $-6.71 \times 10^{10}$                                    | $5.55 \times 10^{11}$                                    | $6.34 \times 10^{11}$                                    |
| $2.55 \times 10^5$    | $2.24 \times 10^{13}$                                 | $-5.96 \times 10^{10}$                                    | $6.09 \times 10^{11}$                                    | $6.67 \times 10^{11}$                                    |
| $5.11 \times 10^5$    | $2.00 \times 10^{13}$                                 | $-5.15 \times 10^{10}$                                    | $5.71 \times 10^{11}$                                    | $6.11 \times 10^{11}$                                    |
| $5.11 \times 10^6$    | $2.51 \times 10^{12}$                                 | $-1.54 \times 10^{10}$                                    | $2.18 \times 10^{11}$                                    | $2.21 \times 10^{11}$                                    |
| $5.11 \times 10^7$    | $7.34 \times 10^{10}$                                 | $-8.22 \times 10^8$                                       | $2.35 \times 10^{10}$                                    | $2.36 \times 10^{10}$                                    |
| $5.11 \times 10^9$    | $9.76 \times 10^6$                                    | $-7.57 \times 10^1$                                       | $3.83 \times 10^6$                                       | $3.84 \times 10^6$                                       |
| $5.11 \times 10^{11}$ | $9.76 \times 10^2$                                    | $-7.57 \times 10^{-7}$                                    | $3.83 \times 10^2$                                       | $3.84 \times 10^2$                                       |
| $5.11 \times 10^{13}$ | $9.76 \times 10^{-2}$                                 | $-7.57 \times 10^{-15}$                                   | $3.83 \times 10^{-2}$                                    | $3.84 \times 10^{-2}$                                    |
| <hr/>                 |                                                       |                                                           |                                                          |                                                          |
|                       | $W_{\text{AV-Ne}} M^2 c^4/(\text{eV}^2 h \text{ Hz})$ | $W_{\text{AV-eN,dia}} M^2 c^4/(\text{eV}^2 h \text{ Hz})$ | $W_{\text{AV-eN,UC}} M^2 c^4/(\text{eV}^2 h \text{ Hz})$ | $W_{\text{AV-eN,CP}} M^2 c^4/(\text{eV}^2 h \text{ Hz})$ |
| $\infty$ (PN)         | $2.55 \times 10^{26}$                                 | 0                                                         | $1.00 \times 10^{26}$                                    | $1.00 \times 10^{26}$                                    |
| $\infty$ (GN)         | $2.1 \times 10^{26}$                                  | $-2.45 \times 10^{24}$                                    | $7.47 \times 10^{25}$                                    | $7.49 \times 10^{25}$                                    |

Table V. Parity-violating matrix elements that mix  $|\Omega\rangle$  and  $|- \Omega\rangle$  states in  $\text{Si}^{17}\text{O}$  from electron- $^{17}\text{O}$  interactions for different boson masses  $M$  at the level of 2c-ZORA-BHandH/dyall.cv4z(aug). In the limits  $M \rightarrow 0$  and  $M \rightarrow \infty$ , results are shown for a Gaussian (GN) and point-like (PN) nuclear charge density distribution. For AV-eN interactions diamagnetic-like expectation value contributions  $W_{\text{AV-eN,dia}}$ , uncoupled  $W_{\text{AV-eN,UC}}$  and coupled-perturbed results  $W_{\text{AV-eN,CP}}$  are shown (see text in Sec.II) for details). Standard Model electroweak contributions to the parity-violating matrix elements  $W_a$  can be obtained from results for  $W_{\text{AV-Ne}}$  (GN) in the limit  $M \rightarrow \infty$  by multiplication with  $\frac{G_F}{\sqrt{2}h^3c^3}$ . For AV-eN interaction matrix elements we used  $\gamma_{^{17}\text{O}} = -0.757516 \mu_N$ .

| $Mc^2/\text{eV}$      | $W_{\text{AV-Ne}}/(h \text{ Hz})$                     | $W_{\text{AV-eN,dia}}/(h \text{ Hz})$                     | $W_{\text{AV-eN,UC}}/(h \text{ Hz})$                     | $W_{\text{AV-eN,CP}}/(h \text{ Hz})$                     |
|-----------------------|-------------------------------------------------------|-----------------------------------------------------------|----------------------------------------------------------|----------------------------------------------------------|
| 0 (GN)                | $9.40 \times 10^{12}$                                 | $1.84 \times 10^8$                                        | $9.95 \times 10^8$                                       | $3.05 \times 10^{10}$                                    |
| 0 (PN)                | $9.40 \times 10^{12}$                                 | $1.84 \times 10^8$                                        | $9.93 \times 10^8$                                       | $3.05 \times 10^{10}$                                    |
| $5.11 \times 10^{-5}$ | $9.40 \times 10^{12}$                                 | $1.84 \times 10^8$                                        | $9.93 \times 10^8$                                       | $3.05 \times 10^{10}$                                    |
| $5.11 \times 10^{-3}$ | $9.40 \times 10^{12}$                                 | $1.84 \times 10^8$                                        | $9.93 \times 10^8$                                       | $3.05 \times 10^{10}$                                    |
| $5.11 \times 10^{-1}$ | $9.40 \times 10^{12}$                                 | $1.84 \times 10^8$                                        | $9.93 \times 10^8$                                       | $3.05 \times 10^{10}$                                    |
| $5.11 \times 10^1$    | $9.42 \times 10^{12}$                                 | $1.84 \times 10^8$                                        | $9.86 \times 10^8$                                       | $3.05 \times 10^{10}$                                    |
| $2.55 \times 10^2$    | $9.67 \times 10^{12}$                                 | $1.84 \times 10^8$                                        | $9.57 \times 10^8$                                       | $3.04 \times 10^{10}$                                    |
| $5.11 \times 10^2$    | $1.02 \times 10^{13}$                                 | $1.84 \times 10^8$                                        | $9.21 \times 10^8$                                       | $3.02 \times 10^{10}$                                    |
| $2.55 \times 10^3$    | $1.05 \times 10^{13}$                                 | $1.85 \times 10^8$                                        | $6.66 \times 10^8$                                       | $2.70 \times 10^{10}$                                    |
| $5.11 \times 10^3$    | $2.77 \times 10^{12}$                                 | $1.83 \times 10^8$                                        | $4.47 \times 10^8$                                       | $2.34 \times 10^{10}$                                    |
| $2.55 \times 10^4$    | $-2.40 \times 10^{13}$                                | $1.45 \times 10^8$                                        | $-1.52 \times 10^8$                                      | $1.11 \times 10^{10}$                                    |
| $5.11 \times 10^4$    | $-2.04 \times 10^{13}$                                | $1.09 \times 10^8$                                        | $-2.62 \times 10^8$                                      | $5.67 \times 10^9$                                       |
| $2.55 \times 10^5$    | $-3.12 \times 10^{12}$                                | $3.55 \times 10^7$                                        | $-1.58 \times 10^8$                                      | $4.06 \times 10^8$                                       |
| $5.11 \times 10^5$    | $-9.63 \times 10^{11}$                                | $1.91 \times 10^7$                                        | $-1.09 \times 10^8$                                      | $5.27 \times 10^7$                                       |
| $5.11 \times 10^6$    | $-1.19 \times 10^{10}$                                | $1.93 \times 10^6$                                        | $-3.75 \times 10^7$                                      | $-3.56 \times 10^7$                                      |
| $5.11 \times 10^7$    | $-1.22 \times 10^8$                                   | $1.05 \times 10^5$                                        | $-7.51 \times 10^6$                                      | $-7.49 \times 10^6$                                      |
| $5.11 \times 10^9$    | $-1.28 \times 10^4$                                   | $3.93 \times 10^{-2}$                                     | $-2.14 \times 10^3$                                      | $-2.14 \times 10^3$                                      |
| $5.11 \times 10^{11}$ | $-1.28$                                               | $3.94 \times 10^{-10}$                                    | $-2.14 \times 10^{-1}$                                   | $-2.14 \times 10^{-1}$                                   |
| $5.11 \times 10^{13}$ | $-1.28 \times 10^{-4}$                                | $3.94 \times 10^{-18}$                                    | $-2.14 \times 10^{-5}$                                   | $-2.14 \times 10^{-5}$                                   |
| <hr/>                 |                                                       |                                                           |                                                          |                                                          |
|                       | $W_{\text{AV-Ne}} M^2 c^4/(\text{eV}^2 h \text{ Hz})$ | $W_{\text{AV-eN,dia}} M^2 c^4/(\text{eV}^2 h \text{ Hz})$ | $W_{\text{AV-eN,UC}} M^2 c^4/(\text{eV}^2 h \text{ Hz})$ | $W_{\text{AV-eN,CP}} M^2 c^4/(\text{eV}^2 h \text{ Hz})$ |
| $\infty$ (PN)         | $-3.34 \times 10^{23}$                                | 0                                                         | $-5.60 \times 10^{22}$                                   | $-5.59 \times 10^{22}$                                   |
| $\infty$ (GN)         | $-3.20 \times 10^{23}$                                | $3.19 \times 10^{20}$                                     | $-4.39 \times 10^{22}$                                   | $-4.39 \times 10^{22}$                                   |

Table VI. Parity-violating matrix elements that mix  $|\Omega\rangle$  and  $|- \Omega\rangle$  states in  $^{29}\text{SiO}^+$  from electron- $^{29}\text{O}$  interactions for different boson masses  $M$  at the level of 2c-ZORA-BHandH/dyall.cv4z(aug). In the limits  $M \rightarrow 0$  and  $M \rightarrow \infty$ , results are shown for a Gaussian (GN) and point-like (PN) nuclear charge density distribution. For AV-eN interactions diamagnetic-like expectation value contributions  $W_{\text{AV-eN,dia}}$ , uncoupled  $W_{\text{AV-eN,UC}}$  and coupled-perturbed results  $W_{\text{AV-eN,CP}}$  are shown (see text in Sec.II) for details). Standard Model electroweak contributions to the parity-violating matrix elements  $W_a$  can be obtained from results for  $W_{\text{AV-Ne}}$  (GN) in the limit  $M \rightarrow \infty$  by multiplication with  $\frac{G_F}{\sqrt{2}h^3c^3}$ . For AV-eN interaction matrix elements we used  $\gamma_{^{29}\text{Si}} = -1.11058 \mu_N$ .

| $Mc^2/\text{eV}$      | $W_{\text{AV-Ne}}/(h \text{ Hz})$                     | $W_{\text{AV-eN,dia}}/(h \text{ Hz})$                     | $W_{\text{AV-eN,UC}}/(h \text{ Hz})$                     | $W_{\text{AV-eN,CP}}/(h \text{ Hz})$                     |
|-----------------------|-------------------------------------------------------|-----------------------------------------------------------|----------------------------------------------------------|----------------------------------------------------------|
| 0 (GN)                | $-4.99 \times 10^{12}$                                | $-1.35 \times 10^9$                                       | $-2.36 \times 10^9$                                      | $-3.33 \times 10^{10}$                                   |
| 0 (PN)                | $-4.99 \times 10^{12}$                                | $-1.35 \times 10^9$                                       | $-2.34 \times 10^9$                                      | $-3.33 \times 10^{10}$                                   |
| $5.11 \times 10^{-5}$ | $-4.99 \times 10^{12}$                                | $-1.35 \times 10^9$                                       | $-2.34 \times 10^9$                                      | $-3.33 \times 10^{10}$                                   |
| $5.11 \times 10^{-3}$ | $-4.99 \times 10^{12}$                                | $-1.35 \times 10^9$                                       | $-2.34 \times 10^9$                                      | $-3.33 \times 10^{10}$                                   |
| $5.11 \times 10^{-1}$ | $-4.99 \times 10^{12}$                                | $-1.35 \times 10^9$                                       | $-2.34 \times 10^9$                                      | $-3.33 \times 10^{10}$                                   |
| $5.11 \times 10^1$    | $-5.00 \times 10^{12}$                                | $-1.35 \times 10^9$                                       | $-2.29 \times 10^9$                                      | $-3.34 \times 10^{10}$                                   |
| $2.55 \times 10^2$    | $-5.27 \times 10^{12}$                                | $-1.35 \times 10^9$                                       | $-2.08 \times 10^9$                                      | $-3.34 \times 10^{10}$                                   |
| $5.11 \times 10^2$    | $-5.93 \times 10^{12}$                                | $-1.35 \times 10^9$                                       | $-1.84 \times 10^9$                                      | $-3.32 \times 10^{10}$                                   |
| $2.55 \times 10^3$    | $-9.99 \times 10^{12}$                                | $-1.36 \times 10^9$                                       | $-2.88 \times 10^8$                                      | $-2.78 \times 10^{10}$                                   |
| $5.11 \times 10^3$    | $-5.56 \times 10^{12}$                                | $-1.35 \times 10^9$                                       | $8.80 \times 10^8$                                       | $-2.38 \times 10^{10}$                                   |
| $2.55 \times 10^4$    | $3.19 \times 10^{13}$                                 | $-1.22 \times 10^9$                                       | $3.47 \times 10^9$                                       | $-1.63 \times 10^{10}$                                   |
| $5.11 \times 10^4$    | $4.13 \times 10^{13}$                                 | $-1.04 \times 10^9$                                       | $3.90 \times 10^9$                                       | $-9.65 \times 10^9$                                      |
| $2.55 \times 10^5$    | $1.27 \times 10^{13}$                                 | $-4.25 \times 10^8$                                       | $2.23 \times 10^9$                                       | $2.12 \times 10^8$                                       |
| $5.11 \times 10^5$    | $4.51 \times 10^{12}$                                 | $-2.42 \times 10^8$                                       | $1.49 \times 10^9$                                       | $8.49 \times 10^8$                                       |
| $5.11 \times 10^6$    | $6.51 \times 10^{10}$                                 | $-2.60 \times 10^7$                                       | $4.35 \times 10^8$                                       | $4.27 \times 10^8$                                       |
| $5.11 \times 10^7$    | $6.90 \times 10^8$                                    | $-1.31 \times 10^6$                                       | $7.31 \times 10^7$                                       | $7.30 \times 10^7$                                       |
| $5.11 \times 10^9$    | $6.93 \times 10^4$                                    | $-3.18 \times 10^{-1}$                                    | $1.73 \times 10^4$                                       | $1.73 \times 10^4$                                       |
| $5.11 \times 10^{11}$ | 6.93                                                  | $-3.19 \times 10^{-9}$                                    | 1.73                                                     | 1.73                                                     |
| $5.11 \times 10^{13}$ | $6.93 \times 10^{-4}$                                 | $-3.19 \times 10^{-17}$                                   | $1.73 \times 10^{-4}$                                    | $1.73 \times 10^{-4}$                                    |
| <hr/>                 |                                                       |                                                           |                                                          |                                                          |
|                       | $W_{\text{AV-Ne}} M^2 c^4/(\text{eV}^2 h \text{ Hz})$ | $W_{\text{AV-eN,dia}} M^2 c^4/(\text{eV}^2 h \text{ Hz})$ | $W_{\text{AV-eN,UC}} M^2 c^4/(\text{eV}^2 h \text{ Hz})$ | $W_{\text{AV-eN,CP}} M^2 c^4/(\text{eV}^2 h \text{ Hz})$ |
| $\infty$ (PN)         | $-3.34 \times 10^{23}$                                | 0                                                         | $-1.40 \times 10^{23}$                                   | $-1.40 \times 10^{23}$                                   |
| $\infty$ (GN)         | $-3.20 \times 10^{23}$                                | $7.98 \times 10^{20}$                                     | $-1.1 \times 10^{23}$                                    | $-1.1 \times 10^{23}$                                    |
